# Supplementary material for: E.T. the Exceptional Trajectories: Text-to-camera-trajectory generation with character awareness
Source: arXiv:2407.01516 source file (2024-07-01)
Supplement: Supplementary file 1 [file supp.tex]

\documentclass[runningheads]{llncs}

% ---------------------------------------------------------------
% Include basic ECCV package
 
% TODO REVIEW: Insert your submission number below by replacing '*****'
% TODO FINAL: Comment out the following line for the camera-ready version
% \usepackage[review,year=2024,ID=632]{eccv}
% TODO FINAL: Un-comment the following line for the camera-ready version
% \usepackage{eccv}

% OPTIONAL: Un-comment the following line for a version which is easier to read
% on small portrait-orientation screens (e.g., mobile phones, or beside other windows)
\usepackage[mobile]{eccv}

% ---------------------------------------------------------------
% Other packages

% Commonly used abbreviations (\eg, \ie, \etc, \cf, \etal, etc.)
\usepackage{eccvabbrv}

% Include other packages here, before hyperref.
\usepackage{graphicx}
\usepackage{booktabs}

% The "axessiblity" package can be found at: https://ctan.org/pkg/axessibility?lang=en
\usepackage[accsupp]{axessibility}  % Improves PDF readability for those with disabilities.

% ---------------------------------------------------------------
% Hyperref package

% It is strongly recommended to use hyperref, especially for the review version.
% Please disable hyperref *only* if you encounter grave issues.
% hyperref with option pagebackref eases the reviewers' job, but should be disabled for the final version.
%
% If you comment hyperref and then uncomment it, you should delete
% main.aux before re-running LaTeX.
% (Or just hit 'q' on the first LaTeX run, let it finish, and you
%  should be clear).

% TODO FINAL: Comment out the following line for the camera-ready version
\usepackage[pagebackref,breaklinks,colorlinks,citecolor=eccvblue]{hyperref}
% TODO FINAL: Un-comment the following line for the camera-ready version
\usepackage{hyperref}

% Support for ORCID icon
\usepackage{orcidlink}

\usepackage{graphicx}
\usepackage{booktabs}
\usepackage{multirow}
\usepackage{tikz}
\usepackage{pgfplots}
\pgfplotsset{compat=newest}
\usepackage{pgfplotstable} % Load the pgfplotstable package for handling data
\usepackage{color}
\usepackage{colortbl}

\definecolor{tabfirst}{rgb}{1, 0.7, 0.7} % red
\definecolor{tabsecond}{rgb}{1, 0.85, 0.7} % orange
\definecolor{tabthird}{rgb}{1, 1, 0.7} % yellow

\definecolor{custompurple}{HTML}{8D57CF}
\definecolor{customgreen}{HTML}{1E945B}
\definecolor{customred}{HTML}{DE333C}
\definecolor{customorange}{HTML}{DD752A}

\definecolor{plotred}{HTML}{e41a1c}
\definecolor{plotblue}{HTML}{377eb8}
\definecolor{plotgreen}{HTML}{4daf4a}
\definecolor{plotpurple}{HTML}{984ea3}

\begin{document}

% ---------------------------------------------------------------
% TODO REVIEW: Replace with your title
\title{
Supplementary material \\
E.T. the Exceptional Trajectories:\\
Text-to-camera-trajectory generation\\ with character awareness
}

% TODO REVIEW: If the paper title is too long for the running head, you can set
% an abbreviated paper title here. If not, comment out.
\titlerunning{Supp - E.T. the Exceptional Trajectories}

% TODO FINAL: Replace with your author list. 
% Include the authors' OCRID for the camera-ready version, if at all possible.
\author{
Robin Courant\inst{1}
Nicolas Dufour\inst{1,2}
Xi Wang\inst{1}
Marc Christie\inst{3}
Vicky Kalogeiton\inst{1}
}

% TODO FINAL: Replace with an abbreviated list of authors.
\authorrunning{R.~Courant et al.}
% First names are abbreviated in the running head.
% If there are more than two authors, 'et al.' is used.

% TODO FINAL: Replace with your institution list.
\institute{
LIX, Ecole Polytechnique, IP Paris \and
LIGM, Ecole des Ponts, CNRS, UGE \and 
Inria, IRISA, CNRS, Univ. Rennes
}

\maketitle

\input{supp/supp_body}

\newpage
% ---- Bibliography ----
%
% BibTeX users should specify bibliography style 'splncs04'.
% References will then be sorted and formatted in the correct style.
%
\bibliographystyle{splncs04}
\bibliography{short_strings,references}
\end{document}
